# Supplementary material for: Transfer Learning of Deep Spatiotemporal Networks to Model Arbitrarily Long Videos of Seizures
Source: arXiv:2106.12014 source file (2021-08-05)
Supplement: Supplementary file 2 [file appendix.tex]

\section*{Appendix}

Appendixes should appear before the acknowledgment.
