# Supplementary material for: Transfer Learning of Deep Spatiotemporal Networks to Model Arbitrarily Long Videos of Seizures
Source: arXiv:2106.12014 source file (2021-08-05)
Supplement: Supplementary file 9 [file newcommands.tex]

\newcommand{\comrem}[1]{}

% https://tex.stackexchange.com/a/71368/216202
\makeatletter
\newcommand*{\org@overidelabel}{}
\let\org@overridelabel\@verridelabel
\@ifpackagelater{acronym}{2015/03/21}{% v1.41
  \renewcommand*{\@verridelabel}[1]{%
    \@bsphack
    \protected@write\@auxout{}{\string\AC@undonewlabel{#1@cref}}%
    \org@overridelabel{#1}%
    \@esphack
  }%
}{% older versions
  \renewcommand*{\@verridelabel}[1]{%
    \@bsphack
    \protected@write\@auxout{}{\string\undonewlabel{#1@cref}}%
    \org@overridelabel{#1}%
    \@esphack
  }%
}
\makeatother
