# Supplementary material for: Transfer Learning of Deep Spatiotemporal Networks to Model Arbitrarily Long Videos of Seizures
Source: arXiv:2106.12014 source file (2021-08-05)
Supplement: Supplementary file 18 [file supplementary.tex]

\section*{Supplementary Material}

We have included as electronic supplementary material six video files (\cref{tab:files}):
\begin{itemize}
    \item Two videos with highly confident predictions: \texttt{ESM\_1.mp4} (true positive, TN) and \texttt{ESM\_2.mp4} (true negative, TN)
    \item Two videos with correct predictions but low confidence due to different predictions between large and small views \texttt{ESM\_3.mp4} (true positive, TN) and \texttt{ESM\_4.mp4} (true negative, TN)
    \item Two videos with incorrect predictions: \texttt{ESM\_5.mp4} and \texttt{ESM\_6.mp4}. Both are false positives (FP).
\end{itemize}

Negative and positive classes represent \acp{fos} and \acp{tcs}, respectively.
Predictions correspond to the model using 16 segments, $\gamma = 4$ and bidirectional long short-term memory (BLSTM) aggregation.
The faces have been blurred to protect the patients' privacy.

\begin{table}
    \setlength{\tabcolsep}{3pt}
    \centering
    \caption{%
        Description of videos included as supplementary material.
        Predictions correspond to the model using 16 segments, $\gamma = 4$  and BLSTM aggregation.
        $\hat{\Yb}_{\text{large}}$: prediction from `large' view.
        $\hat{\Yb}_{\text{small}}$: prediction from `small' (embedded) view.
        $\hat{\Yb}_{\text{mean}}$: mean of $\hat{\Yb}_{\text{large}}$ and $\hat{\Yb}_{\text{small}}$, used for evaluation.
        $\Yb$: annotation for the seizure, where 0 means \ac{fos} and 1 means \ac{tcs}.
        TP: true positive.
        TN: true negative.
        FP: false positive.
        The subject and seizure IDs correspond to the ones in the dataset: \myhref{https://doi.org/10.5522/04/14781771}.
    }
    \label{tab:files}
    \begin{tabular}{cccccccc}
        \toprule
        \textbf{File}       & \textbf{Subject ID} & \textbf{Seizure ID}  & $\hat{\Yb}_{\text{large}}$ & $\hat{\Yb}_{\text{small}}$ & $\hat{\Yb}_{\text{mean}}$ & $\Yb$ & \textbf{Type} \\
        \midrule
        \texttt{ESM\_1.mp4} &                 220 &                   02 &                      1.000 &                      1.000 &                    1.000  &     1 &            TP \\
        \texttt{ESM\_2.mp4} &                 321 &                   11 &                      0.000 &                      0.000 &                    0.000  &     0 &            TN \\
        \texttt{ESM\_3.mp4} &                 321 &                   15 &                      1.000 &                      0.000 &                    0.500  &     1 &            TP \\
        \texttt{ESM\_4.mp4} &                 227 &                   02 &                      0.990 &                      0.000 &                    0.495  &     0 &            TN \\
        \texttt{ESM\_5.mp4} &                 030 &                   04 &                      1.000 &                      0.914 &                    0.957  &     0 &            FP \\
        \texttt{ESM\_6.mp4} &                 199 &                   26 &                      0.809 &                      0.966 &                    0.887  &     0 &            FP \\
        \bottomrule
    \end{tabular}
\end{table}
