# Supplementary material for: Transfer Learning of Deep Spatiotemporal Networks to Model Arbitrarily Long Videos of Seizures
Source: arXiv:2106.12014 source file (2021-08-05)
Supplement: Supplementary file 19 [file packages.tex]

\usepackage{amsmath}
\usepackage{amssymb}                                % fancy math letters
\usepackage{bm}                                     % bold math
\usepackage{booktabs}                               % professional-quality tables
\usepackage{subcaption}                             % for subfigures
\usepackage{comment}                                % add comment environment
\usepackage[nolist]{acronym}                        % acronyms
\usepackage{graphicx}                               % images
\usepackage[utf8]{inputenc}                         % allow utf-8 input
\usepackage{mathtools}                              % for definition symbol :=
\usepackage{siunitx}                                % SI units
\usepackage{xcolor}           % temp

\usepackage{hyperref}
\usepackage[capitalise]{cleveref}                   % needs to be loaded after hyperref
